# Supplementary material for: ROSAR: An Adversarial Re-Training Framework for Robust Side-Scan Sonar Object Detection
Source: arXiv:2410.10554 source file (2024-10-14)
Supplement: Supplementary file 1 [file appendix.tex]

\section{Evaluation Metric Definitions}
\label{sec:eval_metrics}
